# Supplementary material for: Buckling of an elastic ridge: competition between wrinkles and creases
Source: arXiv:1704.01531 source file (2017-04-05)
Supplement: Supplementary file 1 [file SuppMat.pdf]

# Supplementary Material for
# “Buckling of an elastic ridge: competition between wrinkles and creases ”

(Dated: March 21, 2017)

## NUMERICAL METHOD FOR 3-D BIFURCATION ANALYSIS

The numerical method used for the 3-d bifurcation analysis is similar to the one used in [1] for the analysis of a bi-strip system with finite pre-strain. As there is no pre-strain in this problem we do not use the multiplicative decomposition introduced in [1]. Consequently, the invariant solution and the expression of the quadratic forms entering the eigenvalue problem only depend on the loading parameter $\epsilon$. The structure of the resolution is unchanged : we review it briefly in this section.

### Bifurcation analysis

Let $\boldsymbol{\varphi}_1(X,Y,Z)$ denote a small increment of displacement adding up to an invariant solution: using the notations of the main text, $\boldsymbol{\varphi}(X,Y,Z) = \boldsymbol{\varphi}_0^\epsilon(X,Y,Z) + \boldsymbol{\varphi}_1(X,Y,Z) + \cdots$ When linearized, the equilibrium equation (1) takes the classical form

$$\forall \widehat{\boldsymbol{\varphi}}(X,Y,Z), \quad \frac{1}{L}\int_0^{L_0} \left( \iint_{\mathcal{D}} \left[ \widehat{\boldsymbol{F}} : \boldsymbol{\mathcal{L}}_0(\epsilon) : \boldsymbol{F}_1 + \boldsymbol{\Sigma}_0 : \left( \widehat{\boldsymbol{F}}^T \cdot \boldsymbol{F}_1 \right) \right] \mathrm{d}X\,\mathrm{d}Y \right) \mathrm{d}Z = 0. \tag{S.1}$$

Here, $\boldsymbol{F}_1 = \frac{\partial \boldsymbol{\varphi}_1}{\partial(X,Y,Z)}$ is the incremental deformation gradient and $\boldsymbol{\mathcal{L}}_0$ is the tensor of tangent moduli evaluated in the invariant solution,

$$(\mathcal{L}_0)_{ijkl}(\epsilon) = \left[ F_{is}^0 \, \frac{\partial \Sigma_{sj}}{\partial e_{rl}} \, F_{kr}^0 \right]_{\boldsymbol{\varphi}_0^\epsilon}. \tag{S.2}$$

### Material model

A Gent hyperelastic material model is used: the strain energy per unit reference volume has the form

$$W_{3D}(\boldsymbol{E}) = \frac{\mu}{2}\left[ -J_\mathrm{m} \, \ln\left(1 - \frac{I_\mathrm{c} - 3}{J_\mathrm{m}}\right)\right] - \mu \, \ln J + \left(\frac{K}{2} - \frac{\mu}{J_\mathrm{m}}\right) \left(J-1\right)^2 \tag{S.3}$$

where $K$, $\mu$, $J_\mathrm{m}$ are material constants and $I_\mathrm{c} = \boldsymbol{F} : \boldsymbol{F}$, $J = \det \boldsymbol{F}$ are the invariants of the total transformation gradient. The semi-column is a standard notation for the doubly contracted product, $\boldsymbol{A} : \boldsymbol{B} = \mathrm{tr}\big(\boldsymbol{A}^T \cdot \boldsymbol{B}\big)$. In all the numerical simulations we used the following set of material constants: shear modulus $\mu = 1$, bulk modulus $K = 10$ and $J_\mathrm{m} = 100$. The incompressible limit corresponds to $K/\mu \to \infty$. With the set of parameters above, the equivalent Poisson's ratio can be calculated as $\nu \approx 0.45$.

### Pre-stress and tangent moduli

Based on the strain energy per unit reference volume $W_{3D}$ defined in (S.3), the second Piola-Kirchhoff stress tensor $\boldsymbol{\Sigma} = \frac{\partial W_{3D}}{\partial \boldsymbol{E}}$ reads

$$\boldsymbol{\Sigma}(\boldsymbol{\varphi}) = \frac{\mu \, J_\mathrm{m}}{J_\mathrm{m} - I_\mathrm{c} + 3} \, \boldsymbol{1} - \mu \, \boldsymbol{C}^{-1} + \left(K - \frac{2\mu}{J_\mathrm{m}}\right) \, J \left(J-1\right) \boldsymbol{C}^{-1}, \tag{S.4}$$

where $\boldsymbol{C} = \boldsymbol{F}^T \cdot \boldsymbol{F}$ is the Cauchy-Green deformation tensor. For the special case of an invariant solution $\boldsymbol{\varphi}_0^\epsilon$, as defined in (2), the deformation gradients and the stress tensor take the block-diagonal form

$$\boldsymbol{F}_0 = \left[\begin{array}{cc|c} \multicolumn{2}{c|}{\multirow{2}{*}{$\boldsymbol{F}_0^{\parallel}$}} & 0 \\ & & 0 \\ \hline 0 & 0 & 1-\epsilon \end{array}\right] \qquad \boldsymbol{C}_0 = \left[\begin{array}{cc|c} \multicolumn{2}{c|}{\multirow{2}{*}{$\boldsymbol{C}_0^{\parallel}$}} & 0 \\ & & 0 \\ \hline 0 & 0 & (1-\epsilon)^2 \end{array}\right] \qquad \boldsymbol{\Sigma}_0 = \left[\begin{array}{cc|c} \multicolumn{2}{c|}{\multirow{2}{*}{$\boldsymbol{\Sigma}_0^{\parallel}$}} & 0 \\ & & 0 \\ \hline 0 & 0 & \Sigma_0^{\perp} \end{array}\right],$$

where the first two rows and columns correspond to the cross-sectional direction $X$ and $Y$, and the last row and column correspond the axial direction $Z$. The cross-sectional blocks $\boldsymbol{F}_0^{||}$, $\boldsymbol{C}_0^{||}$ and $\boldsymbol{\Sigma}_0^{||}$ depend on the gradients of the cross-sectional displacement $\boldsymbol{\varphi}_0^{||}(\epsilon; X, Y)$. Moreover the blocks $\boldsymbol{\Sigma}_0^{||}$ and $\boldsymbol{\Sigma}_0^{\perp}$ are easily found by identification with (S.4). The tensor of tangent moduli appearing in (S.2) reads, when evaluated in the invariant solution,

$$\boldsymbol{F}_1 : \underline{\underline{\underline{\underline{\mathcal{L}_0}}}}(\lambda) : \widehat{\boldsymbol{F}} = \mathcal{B}_1 \operatorname{tr}(\boldsymbol{F}_1^T \cdot \boldsymbol{F}_0) \operatorname{tr}(\widehat{\boldsymbol{F}}^T \cdot \boldsymbol{F}_0) + \mathcal{B}_2(\boldsymbol{F}_1^T \cdot \boldsymbol{F}_0 \cdot \boldsymbol{C}_0^{-1}) : (\widehat{\boldsymbol{F}}^T \cdot \boldsymbol{F}_0 \cdot \boldsymbol{C}_0^{-1}) \cdots$$
$$+ \mathcal{B}_3 \left[\boldsymbol{C}_0^{-1} : (\boldsymbol{F}_1^T \cdot \boldsymbol{F}_0)\right] \left[\boldsymbol{C}_0^{-1} : (\widehat{\boldsymbol{F}}^T \cdot \boldsymbol{F}_0)\right].$$

The full expressions of the moduli $\mathcal{B}_1$, $\mathcal{B}_2$ and $\mathcal{B}_3$ are

$$\mathcal{B}_1 = \frac{2\,\mu\, J_{\mathrm{m}}}{(J_{\mathrm{m}} - I_{\mathrm{c}}^0 + 3)^2} \quad \mathcal{B}_2 = 2\big(\mu - (K - \frac{2\mu}{J_{\mathrm{m}}})J^0(J^0 - 1)\big) \quad \mathcal{B}_3 = \big(K - \frac{2\mu}{J_{\mathrm{m}}}\big)J^0\big(2\,J^0 - 1\big),$$

where $I_{\mathrm{c}}^0 = \operatorname{tr} \boldsymbol{C}_0$ and $J^0 = \sqrt{\det \boldsymbol{C}_0}$ are the deformation invariants evaluated in the invariant solution $\boldsymbol{\varphi}_0^{\epsilon}$.

## Quadratic forms entering in the eigenvalue problem

Let us consider an arbitrary dependence on $Z$ in the weak form of the linearized equilibrium (S.1): by grouping the terms depending on the total order of derivation with respect to $Z$, one can rewrite the linearized equilibrium as

$$\forall \underline{\widehat{\varphi}}, \quad \frac{1}{L}\int_0^L [K_\epsilon(\widehat{\boldsymbol{\varphi}}, \boldsymbol{\varphi}_1) + \mathcal{C}_\epsilon(\widehat{\boldsymbol{\varphi}}, \boldsymbol{\varphi}_{1,Z}) + \mathcal{C}_\epsilon(\boldsymbol{\varphi}_1, \widehat{\boldsymbol{\varphi}}_{,Z}) + M_\epsilon(\widehat{\boldsymbol{\varphi}}_{,Z}, \boldsymbol{\varphi}_{1,Z})]\,\mathrm{d}Z = 0, \tag{S.5a}$$

where the symbol $Z$ appearing in a subscript after a comma denotes an axial derivative $\partial/\partial Z$. Next, the real and virtual displacements are decomposed into a cross-sectional projection $\boldsymbol{\varphi}_1^{||}$ and $\widehat{\boldsymbol{\varphi}}^{||}$ belonging to the $(XY)$ plane, and an axial component as

$$\boldsymbol{\varphi}_1(X,Y,Z) = \boldsymbol{\varphi}_1^{||}(X,Y,Z) + \varphi_1^{\perp}(X,Y,Z)\,\boldsymbol{e}_z, \qquad \widehat{\boldsymbol{\varphi}}(X,Y,Z) = \widehat{\boldsymbol{\varphi}}^{||}(X,Y,Z) + \widehat{\varphi}^{\perp}(X,Y,Z)\,\boldsymbol{e}_z.$$

The operators in (S.5a) are found by identification with (S.1), they depend on the pre-strain $\epsilon$ through the base solution $\boldsymbol{\varphi}_0^{\epsilon}$, and contain gradients of the displacement with respect to the cross-sectional directions $X$ and $Y$, noted as grad, but *not* with respect to the axial direction $Z$ :

$$K_\epsilon(\widehat{\boldsymbol{\varphi}}, \boldsymbol{\varphi}_1) = k_\epsilon^{||}(\widehat{\boldsymbol{\varphi}}^{||}, \boldsymbol{\varphi}_1^{||}) + k_\epsilon^{\perp}(\widehat{\varphi}^{\perp}, \varphi_1^{\perp}), \tag{S.5b}$$
$$\mathcal{C}_\epsilon(\widehat{\boldsymbol{\varphi}}, \boldsymbol{\varphi}_{1,Z}) = c_\epsilon^1(\widehat{\varphi}^{\perp}, \boldsymbol{\varphi}_{1,Z}^{||}) + c_\epsilon^2(\widehat{\boldsymbol{\varphi}}^{||}, \varphi_{1,Z}^{\perp}), \tag{S.5c}$$
$$M_\epsilon(\widehat{\boldsymbol{\varphi}}_{,Z}, \boldsymbol{\varphi}_{1,Z}) = m_\epsilon^{||}(\widehat{\boldsymbol{\varphi}}_{,Z}^{||}, \boldsymbol{\varphi}_{1,Z}^{||}) + m_\epsilon^{\perp}(\widehat{\varphi}_{,Z}^{\perp}, \varphi_{1,Z}^{\perp}). \tag{S.5d}$$

The detailed expressions of the different 'blocks' are, for the Gent model,

$$k_\epsilon^{||}(\widehat{\boldsymbol{\varphi}}^{||}, \boldsymbol{\varphi}_1^{||}) = \iint_{\mathcal{D}} \Big( \left[(\operatorname{grad}\boldsymbol{\varphi}_1^{||} \cdot \boldsymbol{\Sigma}_0^{||}) : \operatorname{grad}\widehat{\boldsymbol{\varphi}}^{||}\right] + \mathcal{B}_1 \left[\boldsymbol{F}_0^{||} : \operatorname{grad}\boldsymbol{\varphi}_1^{||}\right]\left[\boldsymbol{F}_0^{||} : \operatorname{grad}\widehat{\boldsymbol{\varphi}}^{||}\right] \cdots$$
$$+ \mathcal{B}_2 \left[(\boldsymbol{F}_0^{||})^T \cdot \operatorname{grad}\boldsymbol{\varphi}_1^{||} \cdot (\boldsymbol{C}_0^{||})^{-1}\right] : \left[(\boldsymbol{F}_0^{||})^T \cdot \operatorname{grad}\widehat{\boldsymbol{\varphi}}^{||} \cdot (\boldsymbol{C}_0^{||})^{-1}\right] \cdots$$
$$+ \mathcal{B}_3 \left[(\boldsymbol{C}_0^{||})^{-1} : ((\boldsymbol{F}_0^{||})^T \cdot \operatorname{grad}\boldsymbol{\varphi}_1^{||})\right]\left[(\boldsymbol{C}_0^{||})^{-1} : ((\boldsymbol{F}_0^{||})^T \cdot \operatorname{grad}\widehat{\boldsymbol{\varphi}}^{||})\right] \Big)\mathrm{d}X\,\mathrm{d}Y, \tag{S.5e}$$

$$k_\epsilon^{\perp}(\widehat{\varphi}^{\perp}, \varphi_1^{\perp}) = \iint_{\mathcal{D}} \Big( \left[\boldsymbol{\Sigma}_0^{||} \cdot \operatorname{grad}\varphi_1^{\perp}\right] . \operatorname{grad}\widehat{\varphi}^{\perp} + \frac{\mathcal{B}_2}{2} \operatorname{grad}\widehat{\varphi}^{\perp} . \left[(\boldsymbol{C}_0^{||})^{-1} \cdot \operatorname{grad}\varphi_1^{\perp}\right] \Big)\mathrm{d}X\,\mathrm{d}Y, \tag{S.5f}$$

$$c_\epsilon^1(\widehat{\varphi}^{\perp}, \boldsymbol{\varphi}_{1,Z}^{||}) = \iint_{\mathcal{D}} \frac{\mathcal{B}_2}{2(1-\epsilon)} \operatorname{grad}\widehat{\varphi}^{\perp} . ((\boldsymbol{F}_0^{||})^{-1} \cdot \boldsymbol{\varphi}_{1,Z}^{||})\,\mathrm{d}X\,\mathrm{d}Y, \tag{S.5g}$$

$$c_\epsilon^2(\widehat{\boldsymbol{\varphi}}^{||}, \varphi_{1,Z}^{\perp}) = \iint_{\mathcal{D}} \big(\mathcal{B}_1(1-\epsilon)\,\boldsymbol{F}_0^{||} : \big(\varphi_{,1Z}^{\perp} \operatorname{grad}\widehat{\boldsymbol{\varphi}}_1^{||}\big) + \frac{\mathcal{B}_3}{(1-\epsilon)}(\boldsymbol{F}_0^{||})^{-T} : \big(\varphi_{1,Z}^{\perp} \operatorname{grad}\widehat{\boldsymbol{\varphi}}_1^{||}\big)\big)\mathrm{d}X\,\mathrm{d}Y, \tag{S.5h}$$

$$m_\epsilon^{||}(\widehat{\boldsymbol{\varphi}}_{,Z}^{||}, \boldsymbol{\varphi}_{1,Z}^{||}) = \iint_{\mathcal{D}} \big(\boldsymbol{\Sigma}_0^{\perp}\, \boldsymbol{\varphi}_{1,Z}^{||} \cdot \widehat{\boldsymbol{\varphi}}_{,Z}^{||} + \frac{\mathcal{B}_2}{(1-\epsilon)^2}\,\frac{1}{2}\boldsymbol{\varphi}_{1,Z}^{||} \cdot \widehat{\boldsymbol{\varphi}}_{,Z}^{||}\big)\mathrm{d}X\,\mathrm{d}Y, \tag{S.5i}$$

$$m_\epsilon^{\perp}(\widehat{\varphi}_{,Z}^{\perp}, \varphi_{1,Z}^{\perp}) = \iint_{\mathcal{D}} \big(\boldsymbol{\Sigma}_0^{\perp}\, \varphi_{1,Z}^{\perp}\widehat{\varphi}_{,Z}^{\perp} + \mathcal{B}_1(1-\epsilon)^2\, \varphi_{1,Z}^{\perp}\widehat{\varphi}_{,Z}^{\perp} + \frac{\mathcal{B}_2}{(1-\epsilon)^2}\, \varphi_{1,Z}^{\perp}\widehat{\varphi}_{,Z}^{\perp} + \frac{\mathcal{B}_3}{(1-\epsilon)^2}\varphi_{1,Z}^{\perp}\widehat{\varphi}_{,Z}^{\perp}\big)\mathrm{d}X\,\mathrm{d}Y. \tag{S.5j}$$

With the aim to derive the Fourier form of the eigenvalue problem announced in (2), we now consider displacements that are pure Fourier modes, *i.e.* that depend harmonically on $Z$:

$$\begin{aligned}\boldsymbol{\varphi}_1^{\|}(X,Y,Z) &= \boldsymbol{\xi}^{\|}(X,Y)\,e^{i\,q\,Z}\\ \varphi_1^{\perp}(X,Y,Z) &= i\,\xi^{\perp}(X,Y)\,e^{i\,q\,Z}\\ \widehat{\boldsymbol{\varphi}}^{\|}(X,Y,Z) &= \hat{\boldsymbol{\xi}}^{\|}(X,Y)\,e^{i\,q\,Z}\\ \widehat{\varphi}^{\perp}(X,Y,Z) &= i\,\hat{\xi}^{\perp}(X,Y)\,e^{i\,q\,Z}\end{aligned}$$

For large $L$, the averages over the axial variable $Z$ in equation (S.5a) can be simplified with the help of the identity

$$\frac{1}{L}\int_0^L \Re\big(\boldsymbol{\mathcal{S}}\,e^{i\,q\,z}\big) : \Re\big(\boldsymbol{\mathcal{T}}\,e^{i\,q\,z}\big)\,\mathrm{d}z = \frac{1}{2}\,\Re\big(\boldsymbol{\mathcal{S}} : \boldsymbol{\mathcal{T}}^\dagger\big) \qquad (\text{for } q \neq 0)$$

for any tensors $\boldsymbol{\mathcal{S}}$ and $\boldsymbol{\mathcal{T}}$ of complex amplitudes. Here, $\Re$ denotes the real part, and $\boldsymbol{\mathcal{T}}^\dagger$ is the complex conjugate of $\boldsymbol{\mathcal{T}}$. When this identity is applied to (S.5a), the variable $Z$ disappears, the wavenumber $q$ appears, and one arrives at the eigenproblem announced in (2): $\forall\widehat{\underline{\xi}},\ \widehat{\underline{\xi}}\cdot\big(K_\epsilon + q\,C_\epsilon + q^2\,M_\epsilon\big)\cdot\underline{\xi}_1 = 0$, where the operators $K_\epsilon$ and $M_\epsilon$ are the discrete form of the operators $K_\epsilon$ and $M_\epsilon$ that appeared in (S.5b) and (S.5d), while $C_\epsilon$ is obtained by discretizing the operator

$$C_\epsilon(\hat{\boldsymbol{\xi}},\boldsymbol{\xi}) = c^1_\epsilon(\hat{\xi}^{\perp},\boldsymbol{\xi}^{\|}) - (c^2_\epsilon)^T(\hat{\xi}^{\perp},\boldsymbol{\xi}^{\|}) + (c^1_\epsilon)^T(\hat{\boldsymbol{\xi}}^{\|},\xi^{\perp}) - c^2_\epsilon(\hat{\boldsymbol{\xi}}^{\|},\xi^{\perp}). \tag{S.6}$$

### Numerical implementation

Our implementation makes use of the finite-element library FEniCS [2]. We mesh the cross-section $\mathcal{D}$ with tetrahedrons and set the typical element size at the three vertices of the cross-section. We use coarse elements at the two vertices on the cross-section's basis and fine elements near the tip ; the size of the mesh elements is computed by linearly interpolating these values on an initial mesh made of coarse elements. The incremental displacement $\boldsymbol{\xi}_1$ is discretized using linear Lagrange elements. The corresponding basis of functions are used, together with the known invariant solution $\boldsymbol{\varphi}_0^\epsilon$, to fill in the matrices $K_\epsilon$, $C_\epsilon$ and $M_\epsilon$. The discrete form of the quadratic eigenvalue problem (2) is then solved using the SLEPc library [3]. A two-level orthogonal Arnoldi method is used, see [4] for a review on numerical solution of quadratic eigenvalue problems; it is combined with shift-and-invert preconditioning, allowing one to compute eigenpairs corresponding to small real eigenvalues $q$ more efficiently [5].

## EFFECT OF THE MESH SIZE AT THE SINGULAR RIDGE

The marginal stability curve in the plane $(\epsilon, q)$ is drawn on Fig. S.1(b) for an angle $\phi = 60°$ with $h \approx 1$ and a fine mesh, $e \ll 1$, where $e$ is the typical element size at the tip. The value of the critical strain $\epsilon_\mathrm{c}$ corresponds to the point on the curve of marginal stability with the smallest abscissa (purple dashed line on Fig. S.1(b)). For the modes living on the small wavenumber branch of the marginal stability curve, the wavelength and the lengthscale associated with the decay away from the ridge are both comparable to the dimension of the cross-section $\sim h$, while for the modes living on the large wavenumber branch they are both comparable to the mesh size, see Fig. S.1(c). As there is no intrinsic length-scale near the singular ridge, the numerical mesh size $e$ appears to play a role and the critical strain depends weakly on the mesh size.

To address this point, we regularize the domain by means of a controlled length $r$; as sketched in Fig. S.2(b): we solve the regularized problem, checking that we have achieved convergence with respect to the mesh size $e$ for any value of $r$, and *then* take the limit $r \to 0$. The typical mesh size near the tip $e$ required for numerical convergence was found to be $r/e = 10$ in the numerical simulations in Fig. S.2. The large wave-number branch tends towards a vertical asymptote as $r \to 0$. Moreover we observe that the modes sitting on this branch collapse on the same curve when plotted in terms of the rescaled wavenumber $q\,r$, as shown in Fig. S.2(a'). These modes are similar to one another, as shown on the colormaps of the lateral displacement in Fig. S.2(b–c).

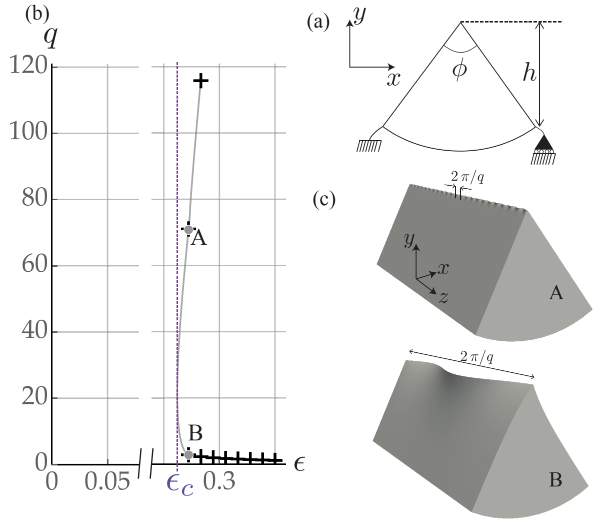


FIG. S.1: (a) Boundary conditions for the linear stability analysis; (b) Wavenumber of critical modes as a function of applied strain for $\phi = 60°$ and $h = 0.866$. The typical mesh size is $e = 0.002$ near the ridge's tip. (c): Eigenmodes corresponding to eigenvalues $A$ and $B$ ($\epsilon = 0.272 \simeq \epsilon_c$).

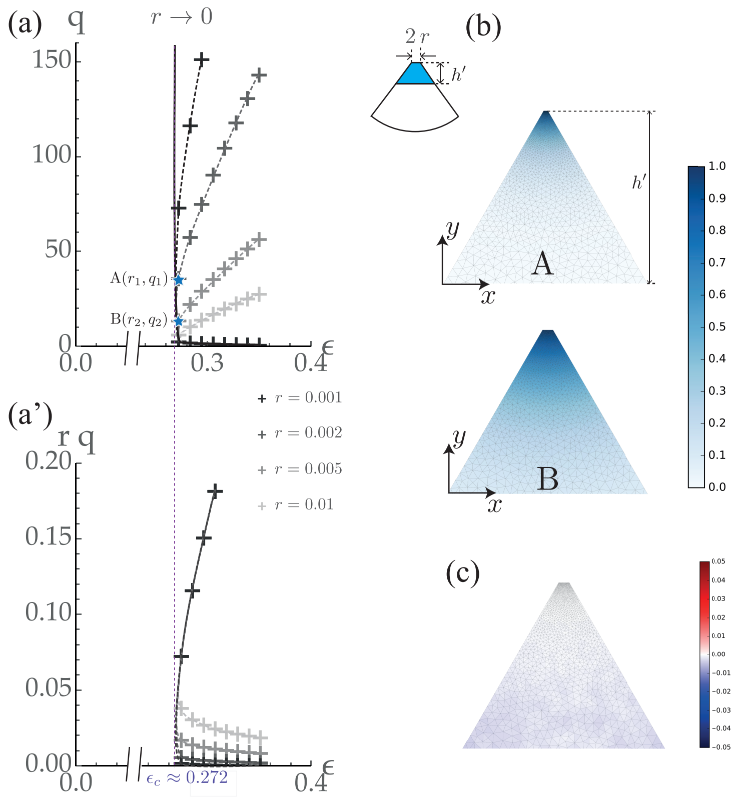


FIG. S.2: (a): Wavenumber of the critical modes as a function of applied strain for various values of regularization parameter $r$ for $\phi = 60°$ and $h = 0.866$. (a'): Same results drawn in plane $(r \times q, \epsilon)$. (b): Colormap of the normalized lateral displacement $\xi_x$ for the first critical mode for two different values of $r$ (corresponding to point A and B on (a)), resp. $r_1 = 0.01$ and $r_2 = 0.005$. Magnification factor, $h' = 0.166$. Inset: sketch of the regularized geometry. (c): Norm of the relative error: $\big(f(\xi_x(r_1)) - \xi_x(r_2)\big)/\xi_x(r_2)$ where $f$ is the homothetic transformation with ratio equal to $q_2/q_1 = r_1/r_2$ and centered at the edge's tip. Magnification factor, $h' = 0.166$.

## NUMERICAL SHOOTING METHOD FOR THE PLATE MODEL

We introduce the new coordinate $\tilde{y} = h - y$. The plate is within the domain $0 < \tilde{y} < h$ and the boundary conditions at the free edge $\tilde{y} = 0$ become

$$w_{,\tilde{y}\tilde{y}} + \nu w_{,zz} = 0 \quad 3\tilde{y}^2 w_{,\tilde{y}\tilde{y}} + \tilde{y}^3 w_{,\tilde{y}\tilde{y}\tilde{y}} + 3\nu\tilde{y}^2 w_{,zz} + (2-\nu)\tilde{y}^3 w_{,zz\tilde{y}} = 0. \tag{S.7a}$$

The boundary conditions at the clamped edge $\tilde{y} \to \infty$ write

$$w = 0 \quad w_{,\tilde{y}} = 0. \tag{S.7b}$$

We consider perturbations that are harmonic in the axial direction $z$. In term of the rescaled coordinate $Y = q\,\tilde{y}$, we denote $\overline{w}(Y)$ the amplitude of the deflection: $w(\tilde{y}) = \overline{w}(Y)\,e^{i\,q\,z}$. Inserting the harmonic deflections into equations (3), (S.7a) and (S.7b) yields a boundary value problem on $\overline{w}(Y)$ that is independent of the wavenumber $q$:

$$-Y^3\,\overline{w}^{(IV)}(Y) - 6\,Y^2\overline{w}^{(III)}(Y) + (2\,Y^3 - 6Y)\,\overline{w}''(Y) + 6\,Y^2\,\overline{w}'(Y) + (Y(6\,\nu + \overline{\sigma}^0) - Y^3)\overline{w}(Y) = 0, \tag{S.8a}$$

$$\overline{w}''(Y) - \nu\overline{w}(Y) = 0 \quad \epsilon\,\overline{w}'''(Y) + (2-\nu)Y\overline{w}'(Y) = 0 \quad \text{for} \quad Y = 0, \tag{S.8b}$$

$$\overline{w}(Y) = 0 \quad \overline{w}'(Y) = 0 \quad \text{for} \quad Y \to \infty. \tag{S.8c}$$

We regularize the geometry by introducing a small parameter $\eta$ as indicated on figure S.3(a): the regularized problem is set between $\eta < \tilde{y}$ and $\tilde{y} < 1/\eta$. The regularized problem will be solved first and then the limit $\eta \to 0$ will provide the result for an *infinite* plate. Equation (S.8a) stays unchanged, boundary conditions (S.8b) and (S.8c) become:

$$\overline{w}''(q\,\eta) - \nu\overline{w}(q\,\eta) = 0 \quad \epsilon\,\overline{w}'''(q\,\eta) + (2-\nu)\eta\,\overline{w}'(q\,\eta) = 0, \tag{S.9a}$$

$$\overline{w}(\frac{q}{\eta}) = 0 \quad \overline{w}'(\frac{q}{\eta}) = 0. \tag{S.9b}$$

For a given value of $q$ the boundary value problem (S.8a), (S.9a) and (S.9b) depends on the Poisson's ratio of the plate $\nu$ and on the dimensionless loading parameter $\overline{\sigma}^0 = \frac{12\,(1-\nu^2)\,\sigma^0}{\phi^2\,E}$. It can be solved by a shooting method as follows. The solution $\overline{w}(Y)$ that satisfy both the differential equation (S.8a) and the boundary conditions (S.9a) and (S.9b) is of dimension $4 - 2 = 2$. Two particular solutions $\overline{w}^1$ and $\overline{w}^2$ spanning this space are found by integrating the differential equation with initial conditions

$$\big((\overline{w}^k), (\overline{w}^k)', (\overline{w}^k)'', (\overline{w}^k)'''\big)_{Y=q\,\eta} = \begin{cases} \big(1, 0, \nu, 0\big) & \text{for first function, } k = 1 \\ \big(0, 1, 0, (2-\nu)\big) & \text{for second function, } k = 2. \end{cases}$$

One can define a $2 \times 2$ shooting matrix $\mathcal{S}(\nu, \eta, \overline{\sigma}^0)$ by filling in the values at $Y = q/\eta$ of the numerical solution $\overline{w}^k$ and their first derivatives. Each column of this matrix is defined by

$$\big(\mathcal{S}(\nu, \eta, \overline{\sigma}^0)\big)_k = \begin{pmatrix} \overline{w}^k \\ \overline{w}^{k\,\prime} \end{pmatrix}_{Y=q/\eta}, \quad k = 1, 2.$$

By construction, this matrix yields $\overline{w}$ and its first derivative at $Y = q/\eta$ in terms of the initial values $\overline{w}(Y = \eta)$ and $\overline{w}'(Y = q\,\eta)$ on the stress-free edge:

$$\begin{pmatrix} \overline{w} \\ \overline{w}' \end{pmatrix}_{Y=q/\eta} = \mathcal{S}(\nu, \eta, \overline{\sigma}^0) \cdot \begin{pmatrix} \overline{w} \\ \overline{w}' \end{pmatrix}_{Y=q\,\eta}.$$

Finally, the boundary condition at $Y = q/\eta$ (S.9b) can be expressed as:

$$\det \mathcal{S}(\nu, \eta, \overline{\sigma}^0) = 0, \tag{S.10}$$

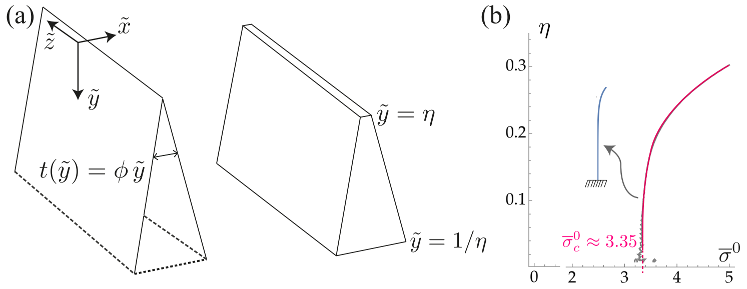


FIG. S.3: (a): Sketch of the thin plate with a varying thickness. (b): Result of implicit equation $\det \mathcal{S}(\nu, \eta, \overline{\sigma}^0) = 0$ for $q = 1$ in plane $(\overline{\sigma}^0, \eta)$ for $\nu = 0.45$ (black line) and critical value $\overline{\sigma}^0_c$ corresponding to the limit $\eta \to 0$ (pink line). Insert: critical mode for $\eta = 0.1$ drawn with an arbitrary amplitude.

which provides an implicit equation for the critical loading parameter $\overline{\sigma}^0$ as a function of Poisson's ratio $\nu$ and of the regularization parameter $\eta$. Note that the wavenumber $q$ has been scaled out from this problem, due to the scale invariance.

The numerical solution of the implicit equation (S.10) is plotted in Fig. S.3(b): for $\nu = 0.45$. $\overline{\sigma}^0$ tends to $\overline{\sigma}^0_c \simeq 3.35$ when the regularization goes to zero, $\eta \to 0$.

[1] C. Lestringant and B. Audoly, Journal of the Mechanics and Physics of Solids (2016).
[2] K. Ølgaard, A. Logg, and G. Wells, SIAM Journal of scientific computing **31**, 849 (2009).
[3] V. Hernandez, J. E. Roman, and V. Vidal, ACM Trans. Math. Software **31**, 351 (2005).
[4] F. Tisseur and K. Meerbergen, SIAM Review **43**, 235 (2001).
[5] Y. Saad, *Numerical methods for large eigenvalue problems* (SIAM, Philadelphia, 2011).
